# Supplementary material for: Equilibrium master equations for time-inconsistent problems with distribution dependent rewards
Source: arXiv:2112.14462 source file (2022-04-08)

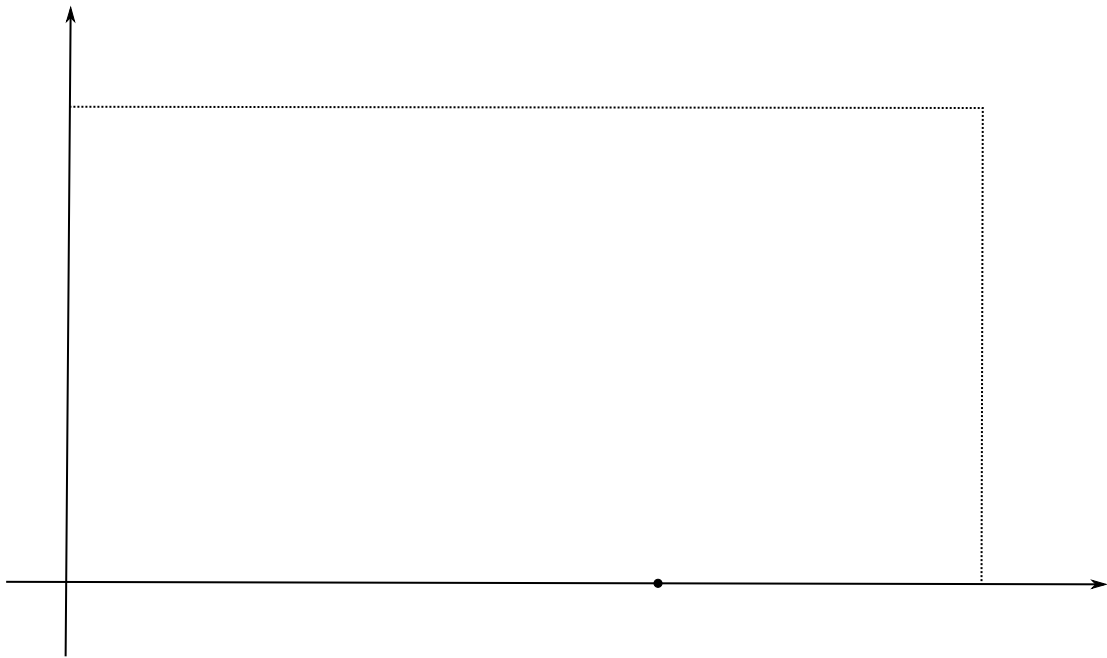

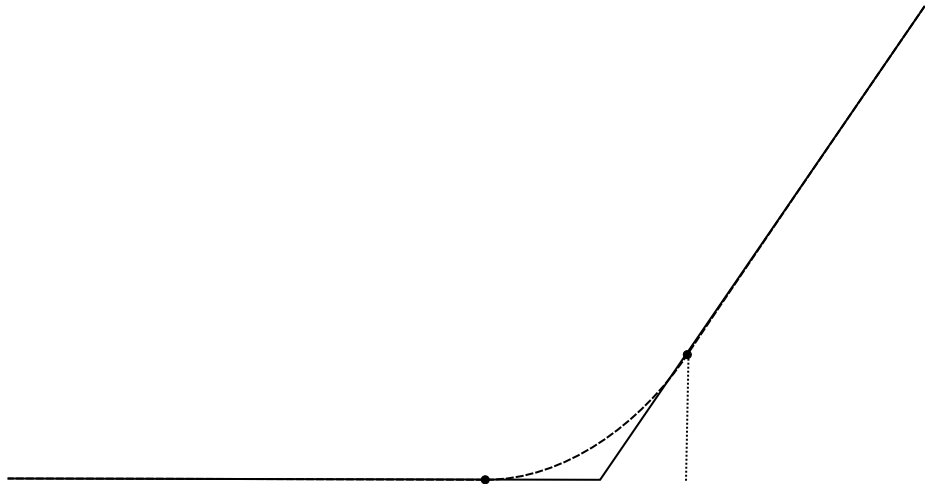

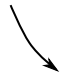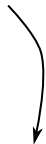

Supplement: Supplementary file 1 [file appendixfigure.pdf]
